# Supplementary material for: Semi-analytical solutions of passive scalar transport in generalized Newtonian fluid flow
Source: arXiv:2505.13320 source file (2025-05-19)
Supplement: Supplementary file 1 [file SI.pdf]

# Supplementary Material: Semi-analytical solutions of passive scalar transport in generalized Newtonian fluid flow

Christopher A. Bowers\*

*The University of North Carolina at Chapel Hill and  
North Carolina State University*

Cass T. Miller

*The University of North Carolina at Chapel Hill*

(Dated: May 19, 2025)

---

\* cabower2@ncsu.edu

TABLE SI. Run index for each pressure drop simulated

| Run Index | Pressure Drop (Pa)      | Run Index | Pressure Drop (Pa)   |
|-----------|-------------------------|-----------|----------------------|
| 1         | $1 \times 10^{-7}$      | 16        | 3.1620               |
| 2         | $3.1620 \times 10^{-7}$ | 17        | 10                   |
| 3         | $1 \times 10^{-6}$      | 18        | 31.620               |
| 4         | $3.1620 \times 10^{-6}$ | 19        | 100                  |
| 5         | $1 \times 10^{-5}$      | 20        | 316.20               |
| 6         | $3.1620 \times 10^{-5}$ | 21        | $1 \times 10^3$      |
| 7         | $1 \times 10^{-4}$      | 22        | $3.1620 \times 10^3$ |
| 8         | $3.1620 \times 10^{-4}$ | 23        | $1 \times 10^4$      |
| 9         | $1 \times 10^{-3}$      | 24        | $3.1620 \times 10^4$ |
| 10        | $3.1620 \times 10^{-3}$ | 25        | $1 \times 10^5$      |
| 11        | $1 \times 10^{-2}$      |           |                      |
| 12        | $3.1620 \times 10^{-2}$ |           |                      |
| 13        | $1 \times 10^{-1}$      |           |                      |
| 14        | $3.1620 \times 10^{-1}$ |           |                      |
| 15        | 1                       |           |                      |

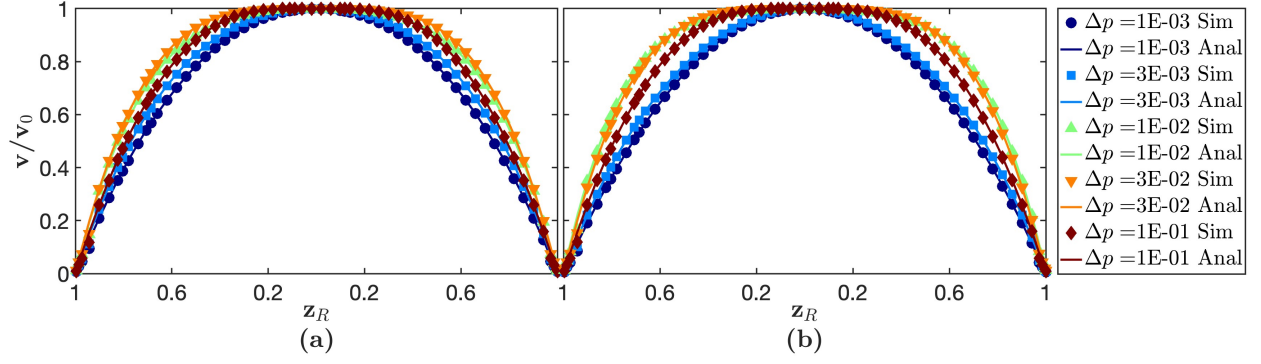

FIG S1. Velocity profiles for (a) Cross and (b) Carreau Fluid 1 flowing through a capillary tube. Pressure drops indicated in the legend have units of Pa.

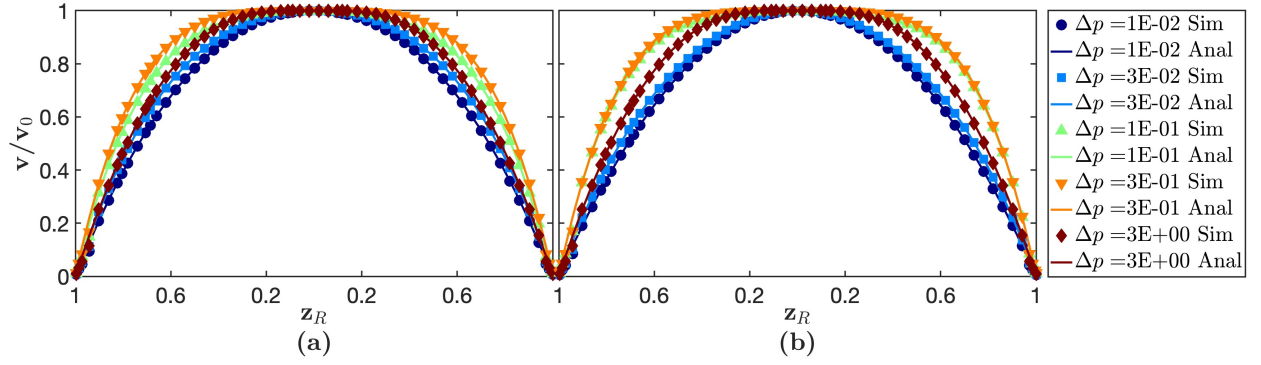

FIG S2. Velocity profiles for (a) Cross and (b) Carreau Fluid 2 flowing through a capillary tube. Pressure drops indicated in the legend have units of Pa.

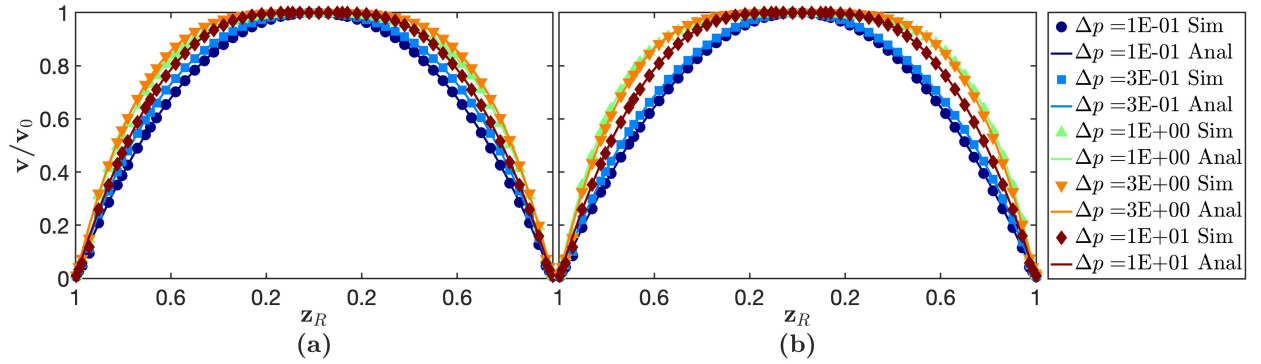

FIG S3. Velocity profiles for (a) Cross and (b) Carreau Fluid 3 flowing through a capillary tube. Pressure drops indicated in the legend have units of Pa.

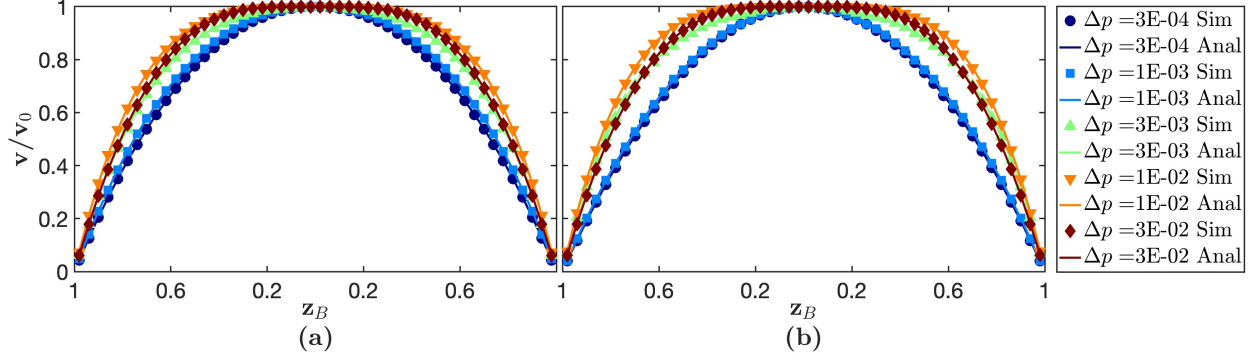

FIG S4. Velocity profiles for (a) Cross and (b) Carreau Fluid 1 flowing through a slit system. Pressure drops indicated in the legend have units of Pa.

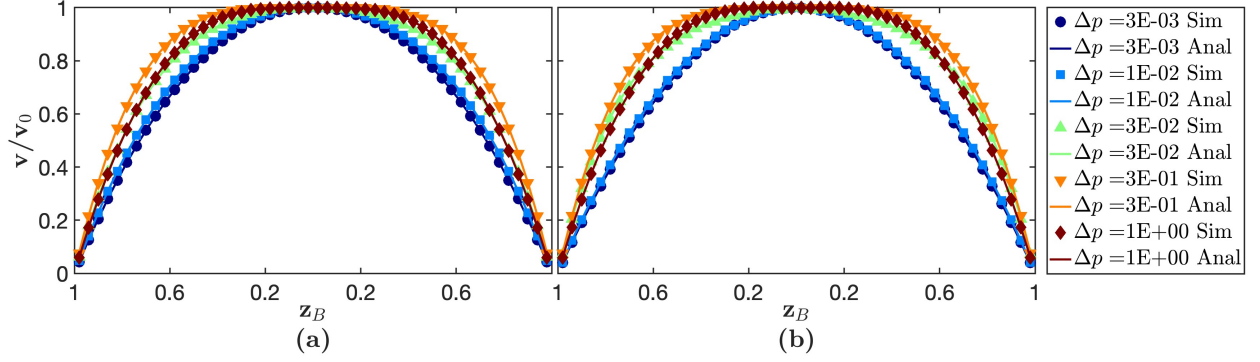

FIG S5. Velocity profiles for (a) Cross and (b) Carreau Fluid 2 flowing through a slit system. Pressure drops indicated in the legend have units of Pa.

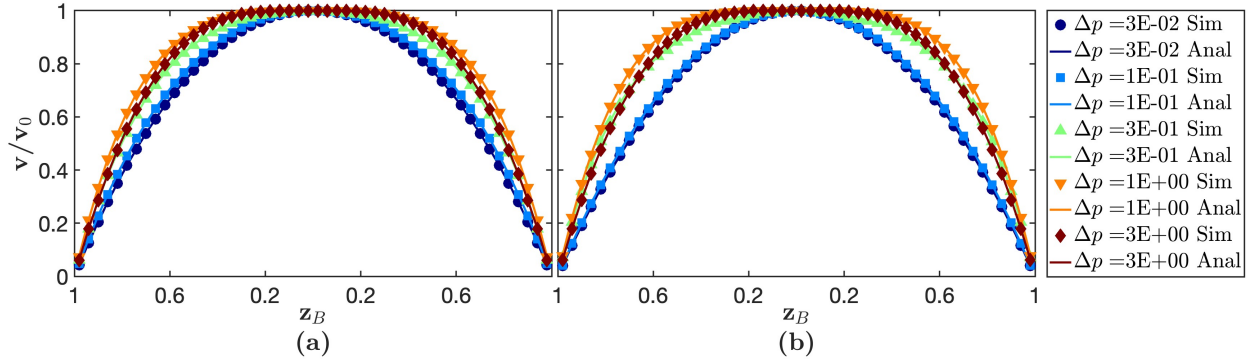

FIG S6. Velocity profiles for (a) Cross and (b) Carreau Fluid 3 flowing through a slit system. Pressure drops indicated in the legend have units of Pa.

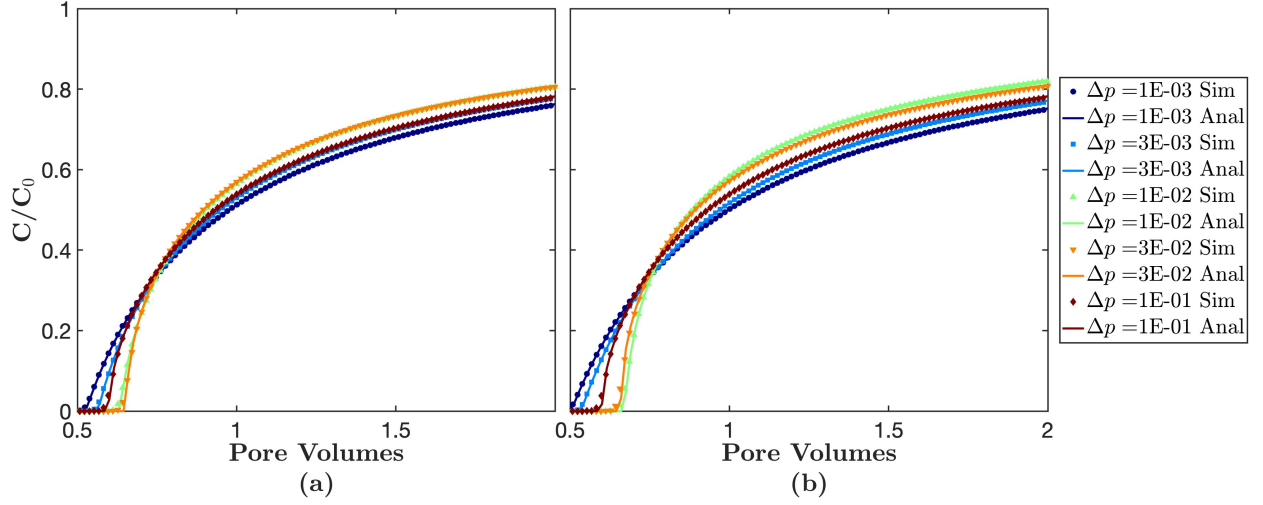

FIG S7. Average effluent concentration for (a) Cross and (b) Carreau Fluid 1 flowing through a capillary tube during advection dominated species transport,  $Pe = 10^5$ . Pressure drops indicated in the legend have units of Pa.

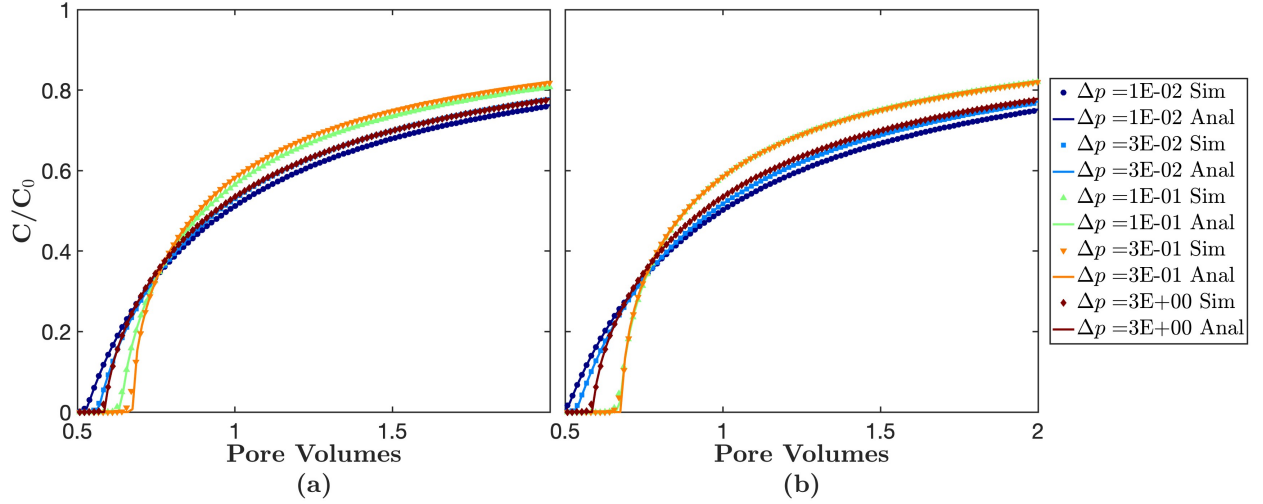

FIG S8. Average effluent concentration for (a) Cross and (b) Carreau Fluid 2 flowing through a capillary tube during advection dominated species transport,  $Pe = 10^5$ . Pressure drops indicated in the legend have units of Pa.

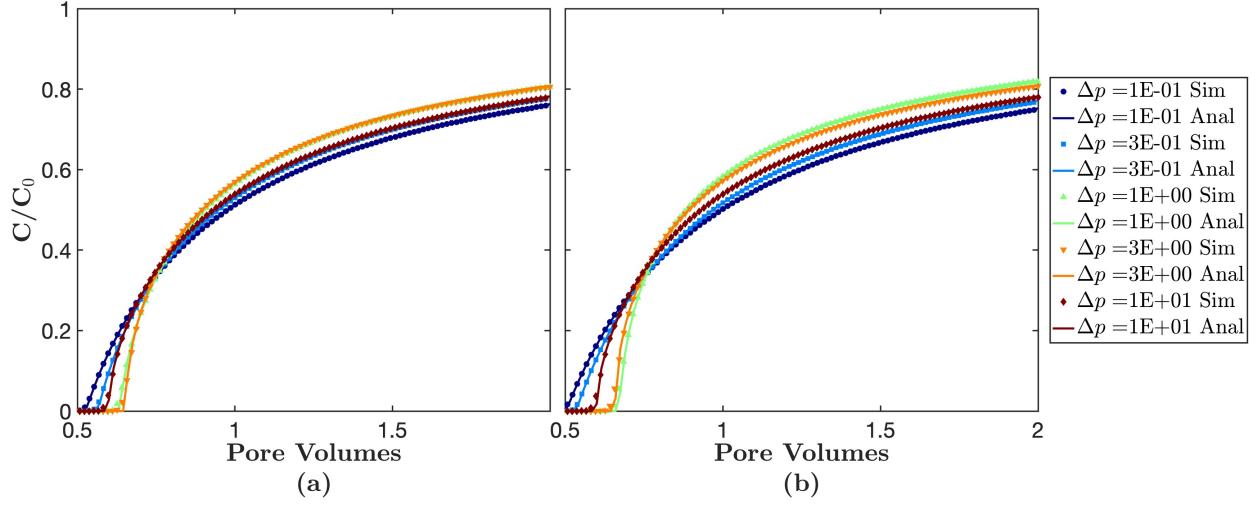

FIG S9. Average effluent concentration for (a) Cross and (b) Carreau Fluid 3 flowing through a capillary tube during advection dominated species transport,  $Pe = 10^5$ . Pressure drops indicated in the legend have units of Pa.

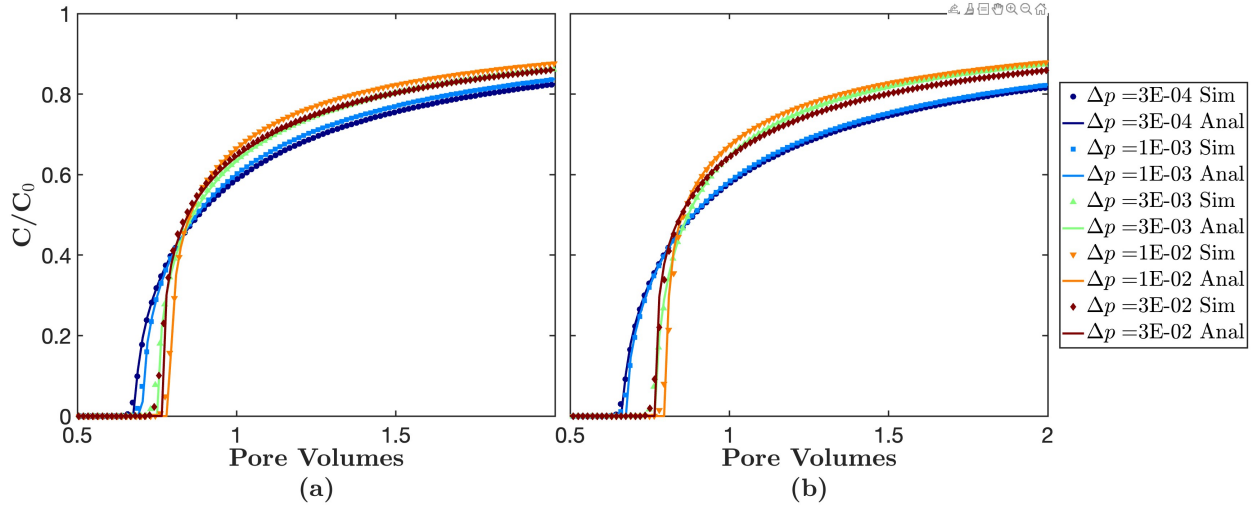

FIG S10. Average effluent concentration for (a) Cross and (b) Carreau Fluid 1 flowing through a slit system during advection dominated species transport,  $Pe = 10^5$ . Pressure drops indicated in the legend have units of Pa.

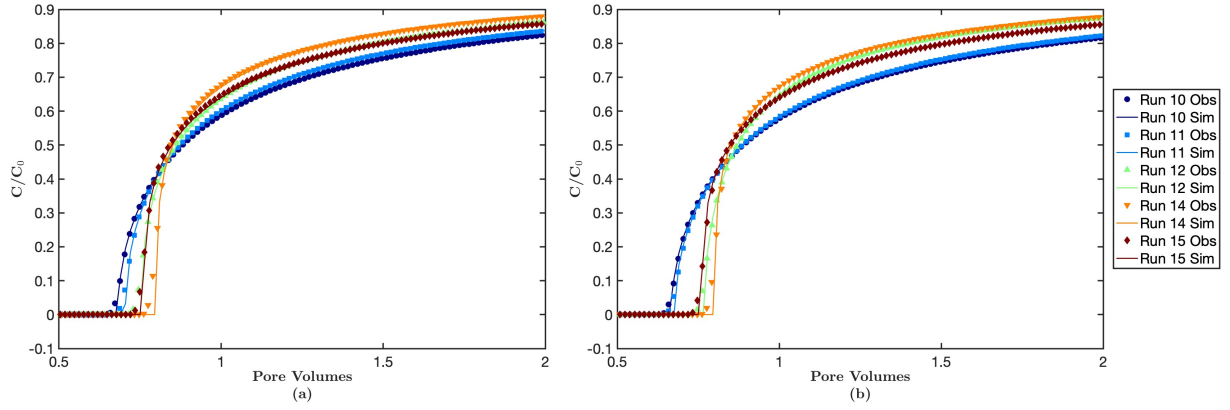

FIG S11. Average effluent concentration for (a) Cross and (b) Carreau Fluid 2 flowing through a slit system during advection dominated species transport,  $Pe = 10^5$ . Pressure drops indicated in the legend have units of Pa.

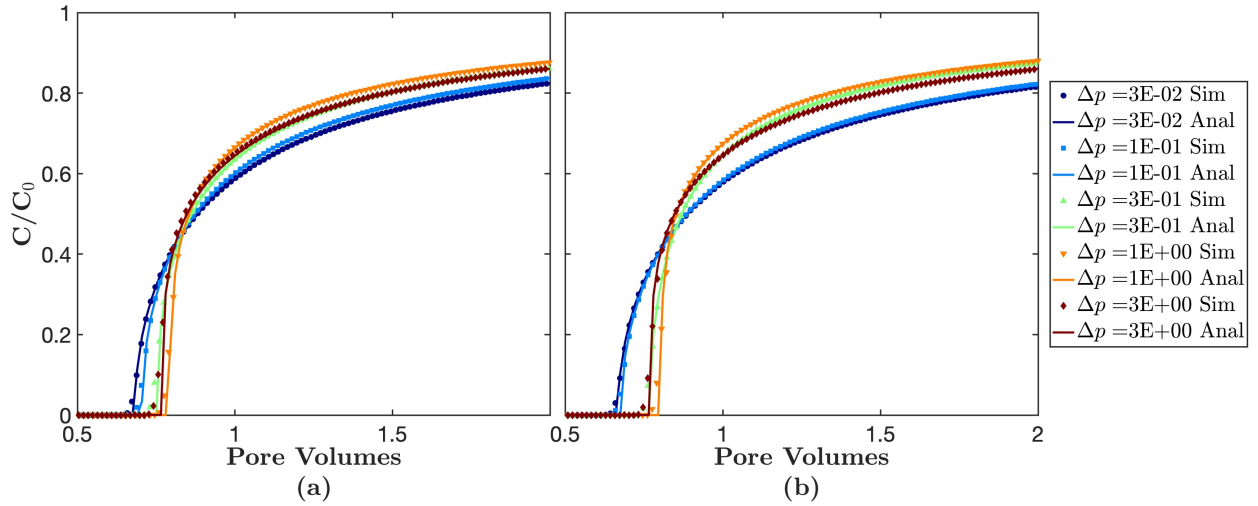

FIG S12. Average effluent concentration for (a) Cross and (b) Carreau Fluid 3 flowing through a slit system during advection dominated species transport,  $Pe = 10^5$ . Pressure drops indicated in the legend have units of Pa.

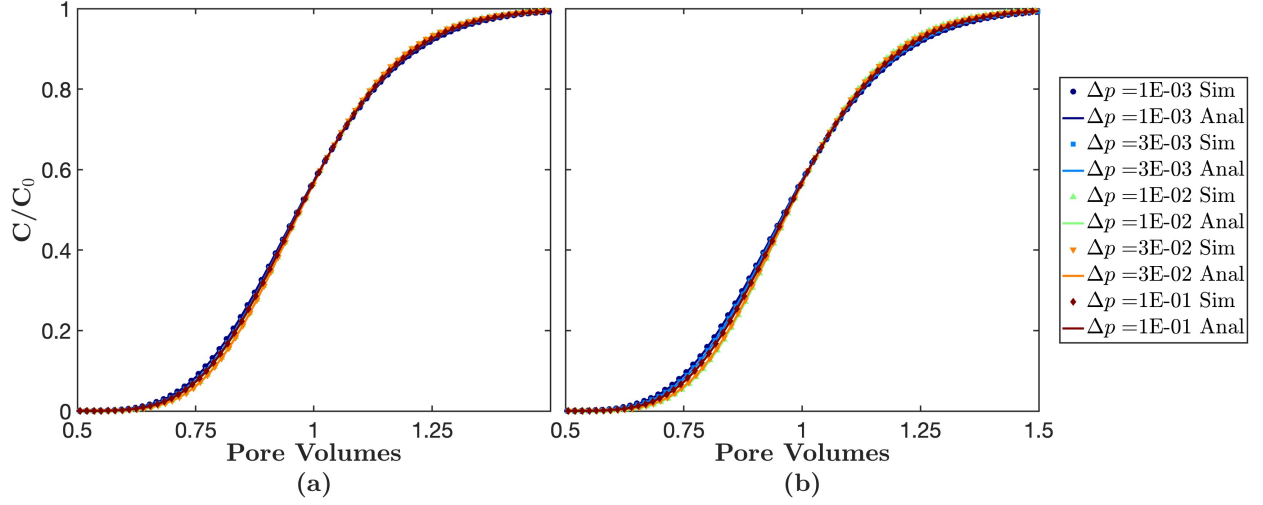

FIG S13. Average effluent concentration for (a) Cross and (b) Carreau Fluid 1 flowing through a capillary tube during enhanced molecular diffusion,  $Pe = 10^2$ . Pressure drops indicated in the legend have units of Pa.

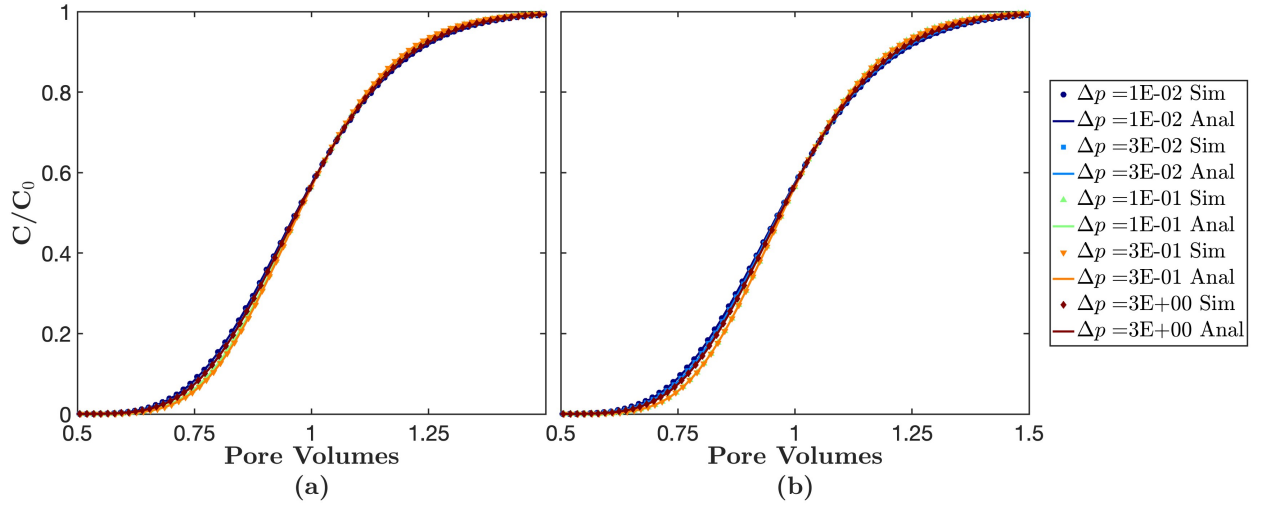

FIG S14. Average effluent concentration for (a) Cross and (b) Carreau Fluid 2 flowing through a capillary tube during enhanced molecular diffusion,  $Pe = 10^2$ . Pressure drops indicated in the legend have units of Pa.



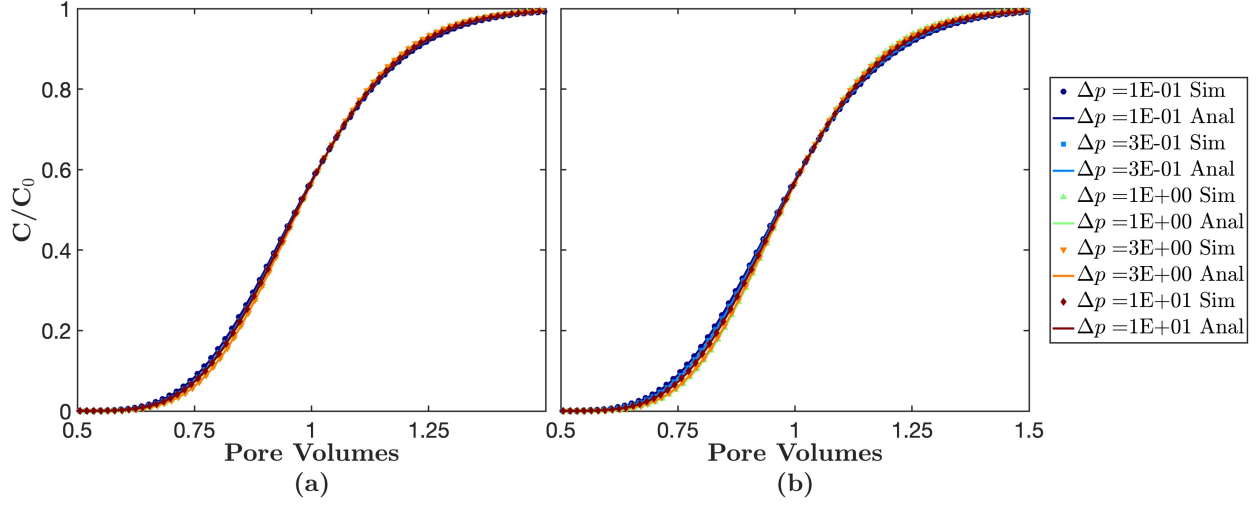

FIG S15. Average effluent concentration for (a) Cross and (b) Carreau Fluid 3 flowing through a capillary tube during enhanced molecular diffusion,  $Pe = 10^2$ . Pressure drops indicated in the legend have units of Pa.

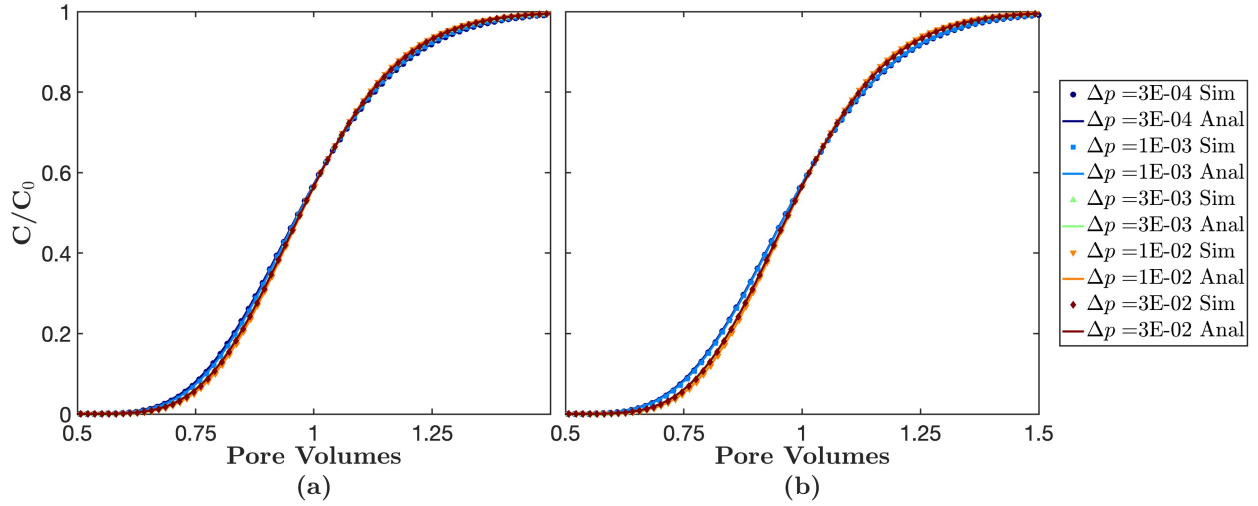

FIG S16. Average effluent concentration for (a) Cross and (b) Carreau Fluid 1 flowing through a slit system during enhanced molecular diffusion,  $Pe = 10^2$ . Pressure drops indicated in the legend have units of Pa.

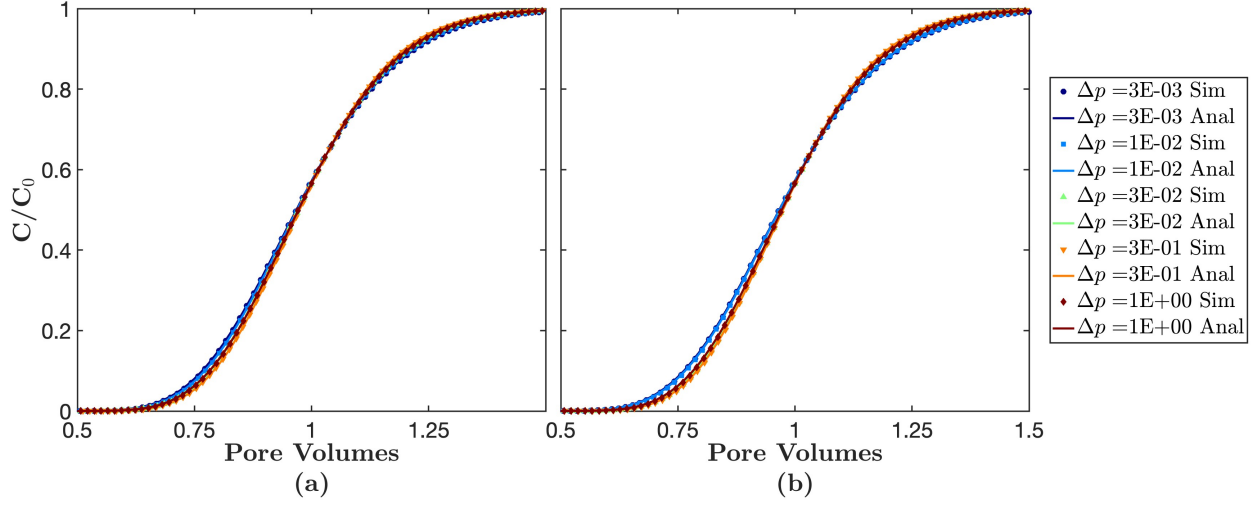

FIG S17. Average effluent concentration for (a) Cross and (b) Carreau Fluid 2 flowing through a slit system during enhanced molecular diffusion,  $Pe = 10^2$ . Pressure drops indicated in the legend have units of Pa.

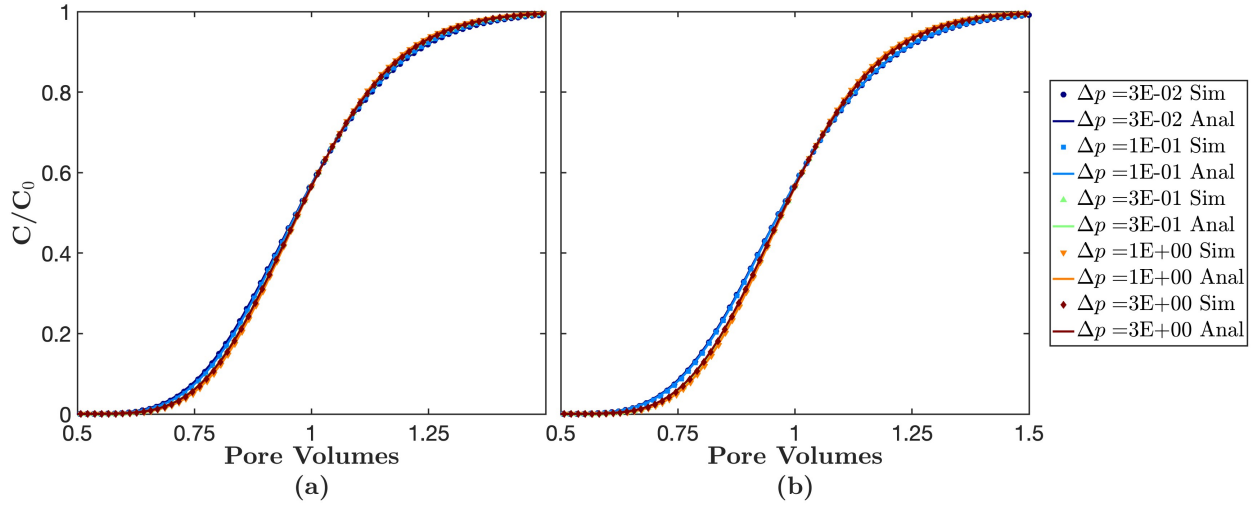

FIG S18. Average effluent concentration for (a) Cross and (b) Carreau Fluid 3 flowing through a slit system during enhanced molecular diffusion,  $Pe = 10^2$ . Pressure drops indicated in the legend have units of Pa.
